# Supplementary material for: Competition between spin-orbit coupling, magnetism, and dimerization in the honeycomb iridates: $\alpha$-Li$_{2}$IrO$_{3}$ under pressure
Source: arXiv:1712.01669 ancillary file (2017-12-05)
Supplement: Supplementary file 1 [file alpha-Li2IrO3_suppl_Hermann.pdf]

# Supplemental Material: Competition between spin-orbit coupling, magnetism, and dimerization in the honeycomb iridates: $\alpha$ -Li<sub>2</sub>IrO<sub>3</sub> under pressure

V. Hermann,<sup>1</sup> M. Altmeyer,<sup>2</sup> J. Ebad-Allah,<sup>1,3</sup> F. Freund,<sup>4</sup> A. Jesche,<sup>4</sup> A. A. Tsirlin,<sup>4</sup> M. Hanfland,<sup>5</sup> P. Gegenwart,<sup>4</sup> I. I. Mazin,<sup>6</sup> D. I. Khomskii,<sup>7</sup> R. Valentí,<sup>2,\*</sup> and C. A. Kuntscher<sup>1,†</sup>

<sup>1</sup>*Experimentalphysik II, Augsburg University, 86159 Augsburg, Germany*

<sup>2</sup>*Institut für Theoretische Physik, Goethe-Universität Frankfurt, 60438 Frankfurt am Main, Germany*

<sup>3</sup>*Department of Physics, Tanta University, 31527 Tanta, Egypt*

<sup>4</sup>*Experimentalphysik VI, Center for Electronic Correlations and Magnetism, Augsburg University, 86159 Augsburg, Germany*

<sup>5</sup>*European Synchrotron Radiation Facility (ESRF), BP 220, 38043 Grenoble, France*

<sup>6</sup>*Code 6393, Naval Research Laboratory, Washington DC 20375, USA*

<sup>7</sup>*II. Physikalisches Institut, Universität zu Köln, 50937 Köln, Germany*

## I. METHODS

### A. Sample Preparation

$\alpha$ -Li<sub>2</sub>IrO<sub>3</sub> single crystals were grown by vapor transport of separated educts as described in Ref. [1] using elemental lithium and iridium as starting materials. The samples were characterized by x-ray diffraction (XRD), specific heat, and magnetic susceptibility measurements, in order to ensure phase-purity and crystal quality. No foreign phases were detected. For the specific sample measured, no indications for significant stacking faults or twinning were observed. The ambient-pressure crystal structure is depicted in Fig. S1.

### B. XRD measurements

The pressure dependence of the lattice parameters at room temperature was determined by single-crystal XRD measurements using synchrotron radiation at beamline ID15B at the European Synchrotron Radiation Facility (ESRF) (Grenoble, France). The wavelength of the radiation was 0.4114 Å, and more than 300 independent reflections were used to determine the crystal structure. Diffraction data were analyzed using the CrysAlisPro software [2], following the established protocols for the beamline [3]. The  $hkl$ -tables were further analyzed using the Jana2006 software [4] to refine the atomic positions. For all pressures only the Ir atoms could be determined via a direct method using SIR 2014 [5]. Also Superflip [6] and shellxt [7] were tried, but did not yield better results. The refinement only converged when fixing all atoms except the Ir atoms to their ambient-pressure positions. Due to the inadequate absorption correction in a diamond anvil cell, we are not able to determine the positions of the weakly absorbing elements Li and O.

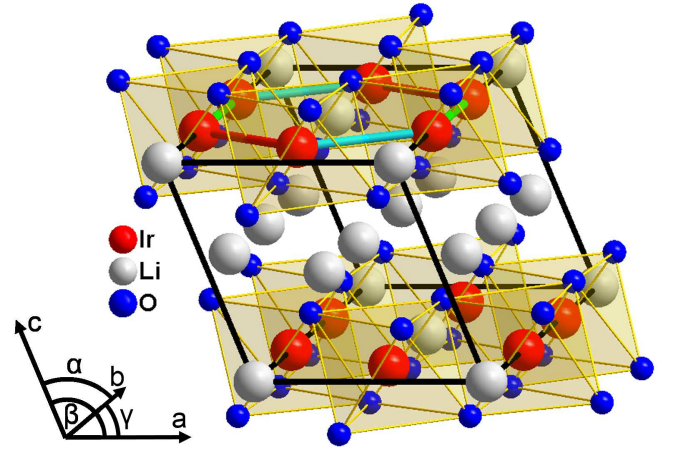

Figure S1. Illustration of the monoclinic unit cell at ambient pressure [1].

### C. Calculations

Density functional theory (DFT) calculations were performed simulating the experimentally accessible pressure range. We employed the PBE [8] generalized gradient approximation (GGA) as implemented in the projector-augmented wave code VASP [9, 10]. Correlation effects were considered within the GGA+U approach [11] and all calculations were performed with inclusion of spin-orbit coupling (SOC). Relaxed structures at finite pressures were obtained by conjugate gradient method, until the forces acting on the ions were less than 0.005 eV/Å. The favorable structures are then identified by comparison of the associated enthalpies. The densities were converged on  $8 \times 6 \times 8$  k meshes.

## II. ADDITIONAL CALCULATIONS

### A. Role of the Hubbard correlation strength

As shown in Fig. S2, at low  $U_{\text{eff}} \sim 0.5$  eV it is not possible to stabilize a non-dimerized, magnetic structure and, interestingly, the Z1 dimerization is energetically fa-

\* valenti@th.physik.uni-frankfurt.de

† christine.kuntscher@physik.uni-augsburg.de

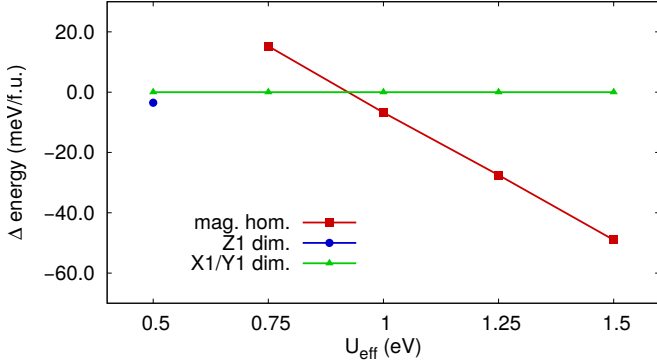

Figure S2. Stability analysis for the homogeneous and X1/Y1 dimerized structure at the experimental ambient-pressure volume in dependence of the Hubbard parameter  $U$ .

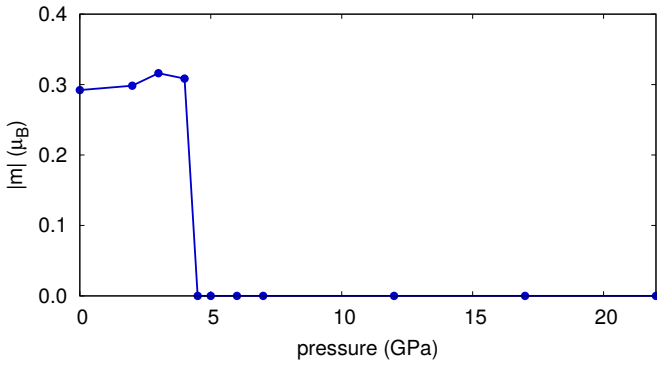

Figure S3. Collapse of the Ir magnetic moments at the transition pressure of approx. 4.5 GPa.

favorable over the experimentally observed X1/Y1 dimerization. For slightly higher values of  $U_{\text{eff}} \sim 0.75$  eV, the homogeneous structure is stabilized by the persistent magnetic moments, but remains higher in energy than the X1/Y1 dimerized structure. Only above values of  $U_{\text{eff}} = 1.0$  eV the high-symmetry  $C2/m$  structure is en-

ergetically favored.

## B. Theoretical predictions: Magnetism

Furthermore, the structural phase transition is accompanied by a sudden collapse of the magnetic moments, as shown in Fig. S3.

## C. Predictions for $\text{Na}_2\text{IrO}_3$

In Fig. S4 we show the evolution of the lattice parameters of  $\text{Na}_2\text{IrO}_3$  up to simulated pressures of 57 GPa. Again, we had to shift the reference point of the simulated pressure by 3 GPa in order to resemble the experimentally measured crystal volume at ambient pressure. Due to the larger central atom in the honeycomb structure, the critical pressure is pushed towards  $\approx 45$  GPa. In contrast to our observations for  $\alpha\text{-Li}_2\text{IrO}_3$  the  $c$  lattice parameters shows a huge jump at the critical pressure, which we can relate to the larger intercalated Na atoms.

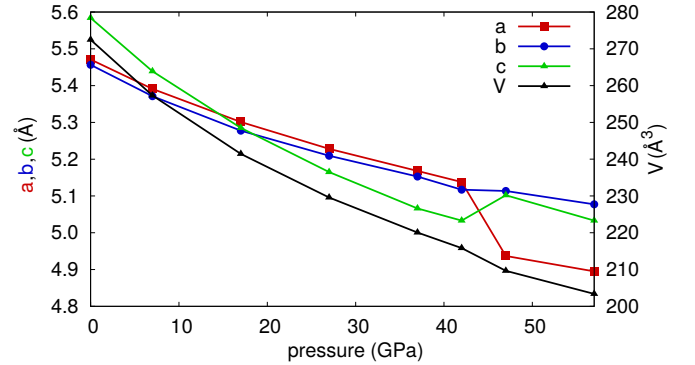

Figure S4. Evolution of the lattice parameters of  $\text{Na}_2\text{IrO}_3$  up to simulated pressures of 57 GPa (corrected by 3 GPa in order to closely resemble the experimental crystal volume at zero pressure).

- 
- [1] F. Freund, S. C. Williams, R. D. Johnson, R. Coldea, P. Gegenwart, and A. Jesche, “Single crystal growth from separated educts and its application to lithium transition-metal oxides,” *Sci. Rep.* **6**, 35362 (2016).
  - [2] Rigaku Oxford Diffraction (2016), CrysAlisPro Software system, version 1.171.38.43a, Rigaku Corporation, Oxford, UK.
  - [3] Marco Merlini and Michael Hanfland, “Single-crystal diffraction at megabar conditions by synchrotron radiation,” *High Press. Res.* **33**, 511–522 (2013).
  - [4] Václav Petříček, Michal Dušek, and Lukáš Palatinus, “Crystallographic Computing System JANA2006: General features,” *Z. Kristallog. Cryst. Mater.* **229**, 345–352 (2014).
  - [5] Maria Cristina Burla, Rocco Caliendo, Benedetta Carrozzini, Giovanni Luca Casciarano, Corrado Cuocci, Carmelo Giacovazzo, Mariarosaria Mallamo, Annamaria Mazzone, and Giampiero Polidori, “Crystal structure determination and refinement via SIR2014,” *J. Appl. Crystallogr.* **48**, 306–309 (2015).
  - [6] Lukáš Palatinus and Gervais Chapuis, “SUPERFLIP – a computer program for the solution of crystal structures by charge flipping in arbitrary dimensions,” *J. Appl. Crystallogr.* **40**, 786–790 (2007).
  - [7] George M. Sheldrick, “A short history of SHELX,” *Acta Crystallogr. Sec. A* **64**, 112–122 (2008).
  - [8] J. P. Perdew, K. Burke, and M. Ernzerhof, “Generalized Gradient Approximation Made Simple,” *Phys. Rev. Lett.* **77**, 3865–3868 (1996).

- [9] J. Hafner, “Ab-initio simulations of materials using VASP: Density-functional theory and beyond,” *J. Comput. Chem.* **29**, 2044–2078 (2008).
- [10] P. E. Blöchl, “Projector augmented-wave method,” *Phys. Rev. B* **50**, 17953–17979 (1994).
- [11] S. L. Dudarev, G. A. Botton, S. Y. Savrasov, C. J. Humphreys, and A. P. Sutton, “Electron-energy-loss spectra and the structural stability of nickel oxide: An LSDA+U study,” *Phys. Rev. B* **57**, 1505–1509 (1998).
